# Supplementary material for: Conductance-based dendrites perform Bayes-optimal cue integration
Source: arXiv:2104.13238 source file (2023-09-20)
Supplement: Supplementary file 1 [file supplements_supplements_raw.tex]

\hrule
\vspace{0.5cm}
{\bf \Huge Drop?}
\vspace{0.5cm}
\hrule

\section{Somatic update reflects Bayesian inference}
%=======================

The intrinsically biderectional somato-dendritic voltage diffusion can be mapped to the Bayesian inversion of a generative distribution as illustrated in Fig.\ref{fig:SI_Fig1}.

In the main text we describe the somatic voltage dynamics (Eqn.~\ref{eq:Cus}) as a stochastic voltage sampling scenario with fixed dendritic input. By virtue of the Gaussian noise $\xi \,$ defined in Eqn.~\ref{eq:results-dynamics-soma}, the somatic voltage $u_s$ stochastically samples around the mean $\bar E_s$ with variance $\lambda_s / \bar g_s$. In this scenario, the fixed presynaptic rates $r$ encode a presynaptic stimulus, and through the dendritic conductances $g^\E_d(r)$ the soma pools the dendritic opinion about how likely the neuronal feature is present in $r$. There is a single prior $p( u_s | \Eprior, \gprior )$ before sampling the dendritic input, a single presynaptic stimulus $r$ generating the pairs $(E_d, g_d)$ for the dendrites $d=1,...,D$, and there is a single posterior $p(\us \,|\, \Eprior, \gprior, E_{\bf d}, g_{\bf d})$.  

There is an alternative scenario that considers stochastic dendritic opinions centered around $E_d$, but endowed with dendrite-specific noise.  In this scenario, the noise $\xi$ in Eqn.~\ref{eq:results-dynamics-soma} is produced by independent dendritic Gaussian noises $\xi_d$, each of variance $2C \lambda_\text{e}\alpha_{sd} \, g_d / \bar g_s$ with $\bargs = \sum_{d=0}^D \alphasd g_{d}$. The noise also includes a somatic contribution $\xi_s$. Hence, we can write $\xi = \sum_{d=0}^D \, \xi_d$. The variance of $\xi$ is the sum of the individual variances, $\mathrm{var}(\xi) = \sum_{d=0}^D \mathrm{var}(\xi_d) = 2C \lambda_\text{e}$. In the stochastic steady state (Eqn.~\ref{eq:ps1}), the somatic voltage fluctuates around $\langle u_s \rangle = \barEs =  \frac{1}{\bargs} \sum_{d=0}^D \alphasd g_{d} E_{d} $ with variance $\sigma_\text{s}^2  =  \lambda_\text{e} / \bargs $. In this dendritic noise scenario, the somatic prior is continuously updated by the new dendritic opinions. It turns into a posterior that is also a prior for the next update.

\section{``On variance''}

\todoin{JJ: moved from methods}
The error in the dendritic estimate $\frac{\lambda_\text{e}}{\bargs}$ of the somatic variance sampled by $(\us^* - \barEs)^2$ vanishes in average when discarding the somatic nudging, $\frac{\lambda_\text{e}}{\bargs} - \langle (\us - \barEs)^2 \rangle = 0$ for $\beta=0$. This is because in the voltage dynamics $\tau \, \dotus =  \barEs - \us + \frac{1}{\bargs}\xi$ with $\tau = C/\bargs$, see Eqn.~\ref{eq:results-dynamics-soma}, the variance $\sigma_I^2 = 2 C\,\lambda_\text{e} /\bargs^2$ in the Gaussian input $\xi/\bargs$ translates into a variance $\sigma_\text{s}^2 = \sigma_I^2 / (2 \tau) = \lambda_\text{e} / \bargs $ of $\us$ \cite{vankampen1992stochastic}. Hence, the total conductance dynamically estimates the voltage variability.
